# Supplementary material for: Speeding-up One-vs-All Training for Extreme Classification via Smart Initialization
Source: arXiv:2109.13122 source file (2021-09-27)
Supplement: Supplementary file 1 [file CmpIterDuration.tex]

% This file was created by tikzplotlib v0.9.6.
\begin{tikzpicture}

\definecolor{color0}{rgb}{0.12156862745098,0.466666666666667,0.705882352941177}
\definecolor{color1}{rgb}{1,0.498039215686275,0.0549019607843137}
\definecolor{color2}{rgb}{0.172549019607843,0.627450980392157,0.172549019607843}

\begin{axis}[
legend cell align={left},
legend style={fill opacity=0.8, draw opacity=1, text opacity=1, draw=white!80!black},
log basis y={10},
tick align=outside,
tick pos=left,
x grid style={white!69.0196078431373!black},
xlabel={iteration},
xmin=0, xmax=15,
xtick style={color=black},
y grid style={white!69.0196078431373!black},
ymin=100000, ymax=1633853.15684273,
ymode=log,
ytick style={color=black},
width=0.5\linewidth,
xmajorgrids,
ymajorgrids
]
\path [draw=color0, fill=color0, opacity=0.2]
(axis cs:0,225321.983945527)
--(axis cs:0,344038.857314788)
--(axis cs:1,467390.949852621)
--(axis cs:2,475216.075525121)
--(axis cs:3,468783.445526141)
--(axis cs:4,462368.112873579)
--(axis cs:5,435858.042158368)
--(axis cs:6,447457.595297406)
--(axis cs:7,461423.60115509)
--(axis cs:8,514133.583313948)
--(axis cs:9,546779.918539638)
--(axis cs:10,542073.317565321)
--(axis cs:11,601149.19185384)
--(axis cs:12,442017.158545047)
--(axis cs:13,508669.774650955)
--(axis cs:14,435921.717121312)
--(axis cs:15,327000.727526457)
--(axis cs:16,332111.359276149)
--(axis cs:17,342266.767843426)
--(axis cs:18,312338.297761552)
--(axis cs:19,315131.293083833)
--(axis cs:20,325129.999961294)
--(axis cs:21,335365.986416007)
--(axis cs:22,308866.003533365)
--(axis cs:22,196366.996466635)
--(axis cs:22,196366.996466635)
--(axis cs:21,201532.013583993)
--(axis cs:20,221786.000038706)
--(axis cs:19,259769.706916167)
--(axis cs:18,238943.702238448)
--(axis cs:17,257998.660728003)
--(axis cs:16,264056.440723851)
--(axis cs:15,254575.772473543)
--(axis cs:14,208674.914457635)
--(axis cs:13,191181.853256022)
--(axis cs:12,218437.319715823)
--(axis cs:11,133719.970936858)
--(axis cs:10,195026.408413326)
--(axis cs:9,171858.408368612)
--(axis cs:8,167326.623440015)
--(axis cs:7,173946.153818385)
--(axis cs:6,168657.924557501)
--(axis cs:5,178424.383216487)
--(axis cs:4,163670.286495364)
--(axis cs:3,170218.963899043)
--(axis cs:2,167512.498754591)
--(axis cs:1,181066.399884813)
--(axis cs:0,225321.983945527)
--cycle;

\path [draw=color1, fill=color1, opacity=0.2]
(axis cs:0,230920.071050038)
--(axis cs:0,328839.073436083)
--(axis cs:1,402543.066139806)
--(axis cs:2,436296.153688131)
--(axis cs:3,437049.087230496)
--(axis cs:4,450816.801958906)
--(axis cs:5,423600.747192884)
--(axis cs:6,430548.557607323)
--(axis cs:7,453965.584889622)
--(axis cs:8,514082.465435521)
--(axis cs:9,585343.583885191)
--(axis cs:10,611614.806271237)
--(axis cs:11,582948.578209273)
--(axis cs:12,621200.888578009)
--(axis cs:13,514811.472247193)
--(axis cs:14,344021.334664389)
--(axis cs:15,334524.237711563)
--(axis cs:16,357747.750338764)
--(axis cs:17,335833.308822927)
--(axis cs:18,320271.396460082)
--(axis cs:19,315956.336881059)
--(axis cs:20,317071.093348331)
--(axis cs:21,309508.256276514)
--(axis cs:22,261638.074567061)
--(axis cs:23,251150.873110634)
--(axis cs:24,258657.984520658)
--(axis cs:25,302847.997540852)
--(axis cs:25,165402.002459148)
--(axis cs:25,165402.002459148)
--(axis cs:24,227229.015479342)
--(axis cs:23,239763.126889366)
--(axis cs:22,249440.925432939)
--(axis cs:21,252206.143723486)
--(axis cs:20,259153.306651669)
--(axis cs:19,242340.463118942)
--(axis cs:18,292423.174968489)
--(axis cs:17,278181.941177073)
--(axis cs:16,266878.694105681)
--(axis cs:15,276921.048002722)
--(axis cs:14,244361.498668945)
--(axis cs:13,175468.992869086)
--(axis cs:12,143202.385931795)
--(axis cs:11,188415.256573336)
--(axis cs:10,157499.904920098)
--(axis cs:9,141830.388358448)
--(axis cs:8,156878.182177122)
--(axis cs:7,172685.256544157)
--(axis cs:6,175777.091953057)
--(axis cs:5,182211.002616654)
--(axis cs:4,165978.724767821)
--(axis cs:3,183515.989900356)
--(axis cs:2,183316.306545962)
--(axis cs:1,206750.609179024)
--(axis cs:0,230920.071050038)
--cycle;
\path [draw=color1, fill=color1, opacity=0.2]
(axis cs:27,305929.561919148)
--(axis cs:27,306030.438080852)
--(axis cs:27,305929.561919148)
--(axis cs:27,305929.561919148)
--cycle;

\path [draw=color2, fill=color2, opacity=0.2]
(axis cs:0,407778.519709028)
--(axis cs:0,596134.89484461)
--(axis cs:1,1562418.24322816)
--(axis cs:2,1243011.43686591)
--(axis cs:3,971615.935083091)
--(axis cs:4,727084.200876551)
--(axis cs:5,536246.978823235)
--(axis cs:6,420057.69188227)
--(axis cs:7,363965.25231529)
--(axis cs:8,342049.867636268)
--(axis cs:9,314630.135563075)
--(axis cs:10,304972.393400589)
--(axis cs:11,279398.205526391)
--(axis cs:12,271454.210969835)
--(axis cs:13,266397.126473243)
--(axis cs:14,265994.528303209)
--(axis cs:15,266585.583732921)
--(axis cs:16,267646.170417115)
--(axis cs:17,267427.768981258)
--(axis cs:18,276877.813781133)
--(axis cs:19,278255.970690076)
--(axis cs:20,278536.288515039)
--(axis cs:21,279434.376262393)
--(axis cs:22,280212.505682436)
--(axis cs:23,305201.696416096)
--(axis cs:24,239785.053737252)
--(axis cs:25,242208.951145721)
--(axis cs:25,213641.048854279)
--(axis cs:25,213641.048854279)
--(axis cs:24,208333.612929415)
--(axis cs:23,216020.58929819)
--(axis cs:22,222279.648163718)
--(axis cs:21,200356.290404274)
--(axis cs:20,195506.135727385)
--(axis cs:19,195910.775072636)
--(axis cs:18,202834.77337483)
--(axis cs:17,198184.061134572)
--(axis cs:16,193451.541957467)
--(axis cs:15,191385.318586124)
--(axis cs:14,191988.403120137)
--(axis cs:13,191374.102216985)
--(axis cs:12,190493.586525975)
--(axis cs:11,190818.136182996)
--(axis cs:10,178516.215356473)
--(axis cs:9,186664.722275215)
--(axis cs:8,185130.252405958)
--(axis cs:7,198415.333692074)
--(axis cs:6,213585.111509596)
--(axis cs:5,233879.669736189)
--(axis cs:4,293841.324369154)
--(axis cs:3,405121.363941665)
--(axis cs:2,645362.380088332)
--(axis cs:1,954762.894506272)
--(axis cs:0,407778.519709028)
--cycle;
\path [draw=color2, fill=color2, opacity=0.2]
(axis cs:27,234887.540375166)
--(axis cs:27,234918.459624834)
--(axis cs:28,236524.351128075)
--(axis cs:29,294078.366652186)
--(axis cs:29,294001.633347814)
--(axis cs:29,294001.633347814)
--(axis cs:28,236455.648871925)
--(axis cs:27,234887.540375166)
--cycle;

\addplot [thick, color0]
table {%
0 284680.420630158
1 324228.674868717
2 321364.287139856
3 319501.204712592
4 313019.199684471
5 307141.212687428
6 308057.759927453
7 317684.877486737
8 340730.103376981
9 359319.163454125
10 368549.862989324
11 367434.581395349
12 330227.239130435
13 349925.813953488
14 322298.315789474
15 290788.25
16 298083.9
17 300132.714285714
18 275641
19 287450.5
20 273458
21 268449
22 252616.5
};
\addlegendentry{$t=-2$}
\addplot [thick, color0, opacity=0.2, dashed, forget plot]
table {%
0 344038.857314788
1 467390.949852621
2 475216.075525121
3 468783.445526141
4 462368.112873579
5 435858.042158368
6 447457.595297406
7 461423.60115509
8 514133.583313948
9 546779.918539638
10 542073.317565321
11 601149.19185384
12 442017.158545047
13 508669.774650955
14 435921.717121312
15 327000.727526457
16 332111.359276149
17 342266.767843426
18 312338.297761552
19 315131.293083833
20 325129.999961294
21 335365.986416007
22 308866.003533365
};
\addplot [thick, color0, opacity=0.2, dashed, forget plot]
table {%
0 225321.983945527
1 181066.399884813
2 167512.498754591
3 170218.963899043
4 163670.286495364
5 178424.383216487
6 168657.924557501
7 173946.153818385
8 167326.623440015
9 171858.408368612
10 195026.408413326
11 133719.970936858
12 218437.319715823
13 191181.853256022
14 208674.914457635
15 254575.772473543
16 264056.440723851
17 257998.660728003
18 238943.702238448
19 259769.706916167
20 221786.000038706
21 201532.013583993
22 196366.996466635
};
\addplot [thick, color1]
table {%
0 279879.572243061
1 304646.837659415
2 309806.230117047
3 310282.538565426
4 308397.763363363
5 302905.874904769
6 303162.82478019
7 313325.420716889
8 335480.323806321
9 363586.98612182
10 384557.355595668
11 385681.917391304
12 382201.637254902
13 345140.23255814
14 294191.416666667
15 305722.642857143
16 312313.222222222
17 307007.625
18 306347.285714286
19 279148.4
20 288112.2
21 280857.2
22 255539.5
23 245457
24 242943.5
25 234125
26 288808
27 305980
};
\addlegendentry{$t=-3$}
\addplot [thick, color1, opacity=0.2, dashed, forget plot]
table {%
0 328839.073436083
1 402543.066139806
2 436296.153688131
3 437049.087230496
4 450816.801958906
5 423600.747192884
6 430548.557607323
7 453965.584889622
8 514082.465435521
9 585343.583885191
10 611614.806271237
11 582948.578209273
12 621200.888578009
13 514811.472247193
14 344021.334664389
15 334524.237711563
16 357747.750338764
17 335833.308822927
18 320271.396460082
19 315956.336881059
20 317071.093348331
21 309508.256276514
22 261638.074567061
23 251150.873110634
24 258657.984520658
25 302847.997540852
26 nan
27 306030.438080852
};
\addplot [thick, color1, opacity=0.2, dashed, forget plot]
table {%
0 230920.071050038
1 206750.609179024
2 183316.306545962
3 183515.989900356
4 165978.724767821
5 182211.002616654
6 175777.091953057
7 172685.256544157
8 156878.182177122
9 141830.388358448
10 157499.904920098
11 188415.256573336
12 143202.385931795
13 175468.992869086
14 244361.498668945
15 276921.048002722
16 266878.694105681
17 278181.941177073
18 292423.174968489
19 242340.463118942
20 259153.306651669
21 252206.143723486
22 249440.925432939
23 239763.126889366
24 227229.015479342
25 165402.002459148
26 nan
27 305929.561919148
};
\addplot [thick, color2]
table {%
0 501956.707276819
1 1258590.56886722
2 944186.908477119
3 688368.649512378
4 510462.762622852
5 385063.324279712
6 316821.401695933
7 281190.293003682
8 263590.060021113
9 250647.428919145
10 241744.304378531
11 235108.170854694
12 230973.898747905
13 228885.614345114
14 228991.465711673
15 228985.451159522
16 230548.856187291
17 232805.915057915
18 239856.293577982
19 237083.372881356
20 237021.212121212
21 239895.333333333
22 251246.076923077
23 260611.142857143
24 224059.333333333
25 227925
26 256548
27 234903
28 236490
29 294040
30 265900
};
\addlegendentry{$t=-1$}
\addplot [thick, color2, opacity=0.2, dashed, forget plot]
table {%
0 596134.89484461
1 1562418.24322816
2 1243011.43686591
3 971615.935083091
4 727084.200876551
5 536246.978823235
6 420057.69188227
7 363965.25231529
8 342049.867636268
9 314630.135563075
10 304972.393400589
11 279398.205526391
12 271454.210969835
13 266397.126473243
14 265994.528303209
15 266585.583732921
16 267646.170417115
17 267427.768981258
18 276877.813781133
19 278255.970690076
20 278536.288515039
21 279434.376262393
22 280212.505682436
23 305201.696416096
24 239785.053737252
25 242208.951145721
26 nan
27 234918.459624834
28 236524.351128075
29 294078.366652186
30 nan
};
\addplot [thick, color2, opacity=0.2, dashed, forget plot]
table {%
0 407778.519709028
1 954762.894506272
2 645362.380088332
3 405121.363941665
4 293841.324369154
5 233879.669736189
6 213585.111509596
7 198415.333692074
8 185130.252405958
9 186664.722275215
10 178516.215356473
11 190818.136182996
12 190493.586525975
13 191374.102216985
14 191988.403120137
15 191385.318586124
16 193451.541957467
17 198184.061134572
18 202834.77337483
19 195910.775072636
20 195506.135727385
21 200356.290404274
22 222279.648163718
23 216020.58929819
24 208333.612929415
25 213641.048854279
26 nan
27 234887.540375166
28 236455.648871925
29 294001.633347814
30 nan
};
\end{axis}
\end{tikzpicture}
