# Supplementary material for: Speeding-up One-vs-All Training for Extreme Classification via Smart Initialization
Source: arXiv:2109.13122 source file (2021-09-27)
Supplement: Supplementary file 2 [file CmpObjective.tex]

% This file was created by tikzplotlib v0.9.6.
\begin{tikzpicture}

\definecolor{color0}{rgb}{0.12156862745098,0.466666666666667,0.705882352941177}
\definecolor{color1}{rgb}{1,0.498039215686275,0.0549019607843137}
\definecolor{color2}{rgb}{0.172549019607843,0.627450980392157,0.172549019607843}

\nextgroupplot[
log basis y={10},
tick align=outside,
tick pos=left,
x grid style={white!69.0196078431373!black},
xlabel={iteration},
xmajorgrids,
xmin=0, xmax=15,
xtick style={color=black},
y grid style={white!69.0196078431373!black},
ylabel={loss},
ymajorgrids,
ymin=1, ymax=17347.5830648474,
ymode=log,
ytick style={color=black}
]
\path [draw=color0, fill=color0, opacity=0.2]
(axis cs:0,23.773591047037)
--(axis cs:0,3057.0838787395)
--(axis cs:1,634.257611016826)
--(axis cs:2,387.903508264016)
--(axis cs:3,304.023697704823)
--(axis cs:4,273.306598429468)
--(axis cs:5,265.190978453316)
--(axis cs:6,321.968075480796)
--(axis cs:7,569.18193830871)
--(axis cs:8,1166.29257719957)
--(axis cs:9,1861.80822905486)
--(axis cs:10,2266.61594688163)
--(axis cs:11,1545.13409526611)
--(axis cs:12,933.303677623899)
--(axis cs:13,465.6747879276)
--(axis cs:14,182.46275054949)
--(axis cs:15,57.6841471778243)
--(axis cs:16,51.2456184663802)
--(axis cs:17,33.8623735198234)
--(axis cs:18,29.1048828351508)
--(axis cs:19,32.8034994531956)
--(axis cs:20,37.8633914372835)
--(axis cs:21,37.8071451743216)
--(axis cs:22,37.7787063034767)
--(axis cs:22,13.5836891979277)
--(axis cs:22,13.5836891979277)
--(axis cs:21,13.5839217965344)
--(axis cs:20,13.5840082929212)
--(axis cs:19,13.1507858911891)
--(axis cs:18,10.1371044747243)
--(axis cs:17,10.970139054883)
--(axis cs:16,7.68453560831422)
--(axis cs:15,6.16392254053754)
--(axis cs:14,4.93202378267766)
--(axis cs:13,6.98876651556853)
--(axis cs:12,12.9854273704227)
--(axis cs:11,15.261239365638)
--(axis cs:10,24.5122375805026)
--(axis cs:9,21.3966518672748)
--(axis cs:8,15.3344536037399)
--(axis cs:7,9.04569427762197)
--(axis cs:6,7.02503946534578)
--(axis cs:5,6.82359895868298)
--(axis cs:4,6.89703889707973)
--(axis cs:3,7.02632841625568)
--(axis cs:2,7.78188565482169)
--(axis cs:1,10.0755759141829)
--(axis cs:0,23.773591047037)
--cycle;

\path [draw=color1, fill=color1, opacity=0.2]
(axis cs:0,27.9909755398677)
--(axis cs:0,2506.05761152852)
--(axis cs:1,664.88611748671)
--(axis cs:2,395.799012699683)
--(axis cs:3,305.014150662512)
--(axis cs:4,273.729022359643)
--(axis cs:5,262.353557754239)
--(axis cs:6,286.573462376636)
--(axis cs:7,461.859765105079)
--(axis cs:8,997.803592773233)
--(axis cs:9,1753.58766841726)
--(axis cs:10,2418.18185439566)
--(axis cs:11,2586.74564247489)
--(axis cs:12,1921.21096908906)
--(axis cs:13,830.506366017674)
--(axis cs:14,202.103892812258)
--(axis cs:15,163.763930580008)
--(axis cs:16,54.7813907774548)
--(axis cs:17,41.9506065722177)
--(axis cs:18,42.8350301848155)
--(axis cs:19,44.6028796113512)
--(axis cs:20,44.5175258827426)
--(axis cs:21,44.496125017661)
--(axis cs:22,30.8337330765643)
--(axis cs:23,30.7741353759734)
--(axis cs:24,30.6843064915994)
--(axis cs:25,30.6708480927245)
--(axis cs:26,30.651555779919)
--(axis cs:27,30.654681993729)
--(axis cs:27,30.6244898649936)
--(axis cs:27,30.6244898649936)
--(axis cs:26,30.6322578645666)
--(axis cs:25,18.2229035374089)
--(axis cs:24,18.261685982886)
--(axis cs:23,18.3397748163628)
--(axis cs:22,18.3413275570679)
--(axis cs:21,12.366760920396)
--(axis cs:20,12.3715583899634)
--(axis cs:19,12.4050733184196)
--(axis cs:18,12.586547806322)
--(axis cs:17,8.60193087319925)
--(axis cs:16,9.28943051743241)
--(axis cs:15,5.12662595933527)
--(axis cs:14,5.8018462378152)
--(axis cs:13,7.20517448766934)
--(axis cs:12,12.235196293203)
--(axis cs:11,17.9991701968823)
--(axis cs:10,20.6050807387077)
--(axis cs:9,16.9172722669952)
--(axis cs:8,10.5831151548683)
--(axis cs:7,7.03573630797369)
--(axis cs:6,6.36169804514018)
--(axis cs:5,6.80825102081395)
--(axis cs:4,6.91963523409955)
--(axis cs:3,7.12329583477637)
--(axis cs:2,8.092566724146)
--(axis cs:1,11.2093503805284)
--(axis cs:0,27.9909755398677)
--cycle;

\path [draw=color2, fill=color2, opacity=0.2]
(axis cs:0,588.846911721123)
--(axis cs:0,16521.6565989764)
--(axis cs:1,1637.65608153987)
--(axis cs:2,661.599387610599)
--(axis cs:3,475.48556882805)
--(axis cs:4,385.391120019314)
--(axis cs:5,328.245466799782)
--(axis cs:6,293.263276806706)
--(axis cs:7,268.878941599788)
--(axis cs:8,247.881228522603)
--(axis cs:9,222.574255761049)
--(axis cs:10,177.666273768093)
--(axis cs:11,128.265489135817)
--(axis cs:12,83.4932479482398)
--(axis cs:13,51.408733816474)
--(axis cs:14,35.996714236551)
--(axis cs:15,31.1587050055765)
--(axis cs:16,35.3454023932944)
--(axis cs:17,44.1552177060698)
--(axis cs:18,46.7925182642555)
--(axis cs:19,48.0722940927122)
--(axis cs:20,55.7570033396319)
--(axis cs:21,79.4435288304939)
--(axis cs:22,107.657106935267)
--(axis cs:23,208.828472921037)
--(axis cs:24,24.9295397462075)
--(axis cs:25,24.8762548668398)
--(axis cs:26,24.9212503271258)
--(axis cs:27,24.9082912129071)
--(axis cs:28,24.8655532859607)
--(axis cs:29,24.8635860466122)
--(axis cs:29,24.8317187240007)
--(axis cs:29,24.8317187240007)
--(axis cs:28,24.8353786793924)
--(axis cs:27,24.8745439374083)
--(axis cs:26,24.8944808589)
--(axis cs:25,15.7672812252166)
--(axis cs:24,15.7681311524138)
--(axis cs:23,16.2338741546994)
--(axis cs:22,8.59426751696835)
--(axis cs:21,7.30584592843718)
--(axis cs:20,5.48024427793125)
--(axis cs:19,5.12982154592368)
--(axis cs:18,3.90430839172056)
--(axis cs:17,3.18551219991616)
--(axis cs:16,3.12728155686211)
--(axis cs:15,3.19228684462392)
--(axis cs:14,3.66629564268209)
--(axis cs:13,4.82773208507616)
--(axis cs:12,6.00836820449079)
--(axis cs:11,6.8398421721665)
--(axis cs:10,7.22162598074144)
--(axis cs:9,7.4351926345449)
--(axis cs:8,7.69148853115434)
--(axis cs:7,8.13347187893556)
--(axis cs:6,8.7759714830641)
--(axis cs:5,9.75628936281105)
--(axis cs:4,11.3115955328804)
--(axis cs:3,14.1802418876495)
--(axis cs:2,23.9416092677443)
--(axis cs:1,65.9011965580084)
--(axis cs:0,588.846911721123)
--cycle;

\addplot [thick, color0]
table {%
0 269.588319349416
1 79.9406699305699
2 54.9419761786446
3 46.2187228988266
4 43.4166585563259
5 42.538886732332
6 47.5587892700604
7 71.7540647091499
8 133.732791092735
9 199.590737562429
10 235.711324704008
11 153.559959884941
12 110.087906330957
13 57.0481582964156
14 29.9985103823984
15 18.8563149905032
16 19.8443639322348
17 19.2736853310634
18 17.1767062623931
19 20.7699734662978
20 22.6789907906454
21 22.6620675005218
22 22.6533486426669
};
\addplot [thick, color0, opacity=0.2, dashed, forget plot]
table {%
0 3057.0838787395
1 634.257611016826
2 387.903508264016
3 304.023697704823
4 273.306598429468
5 265.190978453316
6 321.968075480796
7 569.18193830871
8 1166.29257719957
9 1861.80822905486
10 2266.61594688163
11 1545.13409526611
12 933.303677623899
13 465.6747879276
14 182.46275054949
15 57.6841471778243
16 51.2456184663802
17 33.8623735198234
18 29.1048828351508
19 32.8034994531956
20 37.8633914372835
21 37.8071451743216
22 37.7787063034767
};
\addplot [thick, color0, opacity=0.2, dashed, forget plot]
table {%
0 23.773591047037
1 10.0755759141829
2 7.78188565482169
3 7.02632841625568
4 6.89703889707973
5 6.82359895868298
6 7.02503946534578
7 9.04569427762197
8 15.3344536037399
9 21.3966518672748
10 24.5122375805026
11 15.261239365638
12 12.9854273704227
13 6.98876651556853
14 4.93202378267766
15 6.16392254053754
16 7.68453560831422
17 10.970139054883
18 10.1371044747243
19 13.1507858911891
20 13.5840082929212
21 13.5839217965344
22 13.5836891979277
};
\addplot [thick, color1]
table {%
0 264.852784213785
1 86.330420212447
2 56.5953171174373
3 46.6122948261735
4 43.5213164749805
5 42.2630911954446
6 42.697702928735
7 57.0045920829367
8 102.761229674719
9 172.237974995818
10 223.21924726757
11 215.775983545318
12 153.317948484381
13 77.3559518090077
14 34.2428928415899
15 28.9750999603841
16 22.5585443518743
17 18.9962158816695
18 23.2194994607211
19 23.522372154854
20 23.4680883506744
21 23.4578971772293
22 23.780908270385
23 23.7569087417454
24 23.6716532957083
25 23.6413177763897
26 30.6419053030425
27 30.6395822104603
};
\addplot [thick, color1, opacity=0.2, dashed, forget plot]
table {%
0 2506.05761152852
1 664.88611748671
2 395.799012699683
3 305.014150662512
4 273.729022359643
5 262.353557754239
6 286.573462376636
7 461.859765105079
8 997.803592773233
9 1753.58766841726
10 2418.18185439566
11 2586.74564247489
12 1921.21096908906
13 830.506366017674
14 202.103892812258
15 163.763930580008
16 54.7813907774548
17 41.9506065722177
18 42.8350301848155
19 44.6028796113512
20 44.5175258827426
21 44.496125017661
22 30.8337330765643
23 30.7741353759734
24 30.6843064915994
25 30.6708480927245
26 30.651555779919
27 30.654681993729
};
\addplot [thick, color1, opacity=0.2, dashed, forget plot]
table {%
0 27.9909755398677
1 11.2093503805284
2 8.092566724146
3 7.12329583477637
4 6.91963523409955
5 6.80825102081395
6 6.36169804514018
7 7.03573630797369
8 10.5831151548683
9 16.9172722669952
10 20.6050807387077
11 17.9991701968823
12 12.235196293203
13 7.20517448766934
14 5.8018462378152
15 5.12662595933527
16 9.28943051743241
17 8.60193087319925
18 12.586547806322
19 12.4050733184196
20 12.3715583899634
21 12.366760920396
22 18.3413275570679
23 18.3397748163628
24 18.261685982886
25 18.2229035374089
26 30.6322578645666
27 30.6244898649936
};
\addplot [thick, color2]
table {%
0 3119.0906470996
1 328.517115724549
2 125.856084596462
3 82.1127297078132
4 66.025665249373
5 56.5902620256317
6 50.7313527740547
7 46.7645090890499
8 43.664351893393
9 40.6802466447029
10 35.8195390610373
11 29.6195155568879
12 22.3977270333815
13 15.7539707280079
14 11.488019696899
15 9.97334066824248
16 10.51356385934
17 11.8598897420102
18 13.5163760575411
19 15.7035757074233
20 17.4803317619149
21 24.0915375525711
22 30.4176589681809
23 58.2245236074814
24 19.8265542212335
25 19.8048202798113
26 24.9078619967369
27 24.8914118559237
28 24.8504614027475
29 24.8476472765424
30 24.8362636864164
};
\addplot [thick, color2, opacity=0.2, dashed, forget plot]
table {%
0 16521.6565989764
1 1637.65608153987
2 661.599387610599
3 475.48556882805
4 385.391120019314
5 328.245466799782
6 293.263276806706
7 268.878941599788
8 247.881228522603
9 222.574255761049
10 177.666273768093
11 128.265489135817
12 83.4932479482398
13 51.408733816474
14 35.996714236551
15 31.1587050055765
16 35.3454023932944
17 44.1552177060698
18 46.7925182642555
19 48.0722940927122
20 55.7570033396319
21 79.4435288304939
22 107.657106935267
23 208.828472921037
24 24.9295397462075
25 24.8762548668398
26 24.9212503271258
27 24.9082912129071
28 24.8655532859607
29 24.8635860466122
30 nan
};
\addplot [thick, color2, opacity=0.2, dashed, forget plot]
table {%
0 588.846911721123
1 65.9011965580084
2 23.9416092677443
3 14.1802418876495
4 11.3115955328804
5 9.75628936281105
6 8.7759714830641
7 8.13347187893556
8 7.69148853115434
9 7.4351926345449
10 7.22162598074144
11 6.8398421721665
12 6.00836820449079
13 4.82773208507616
14 3.66629564268209
15 3.19228684462392
16 3.12728155686211
17 3.18551219991616
18 3.90430839172056
19 5.12982154592368
20 5.48024427793125
21 7.30584592843718
22 8.59426751696835
23 16.2338741546994
24 15.7681311524138
25 15.7672812252166
26 24.8944808589
27 24.8745439374083
28 24.8353786793924
29 24.8317187240007
30 nan
};
\end{axis}
\end{tikzpicture}
