# Supplementary material for: Speeding-up One-vs-All Training for Extreme Classification via Smart Initialization
Source: arXiv:2109.13122 source file (2021-09-27)
Supplement: Supplementary file 3 [file CmpShift.tex]

% This file was created by tikzplotlib v0.9.6.
\begin{tikzpicture}

\definecolor{color0}{rgb}{0.12156862745098,0.466666666666667,0.705882352941177}
\definecolor{color1}{rgb}{1,0.498039215686275,0.0549019607843137}
\definecolor{color2}{rgb}{0.172549019607843,0.627450980392157,0.172549019607843}

\end{axis}

\draw ({$(current bounding box.south west)!0.5!(current bounding box.south east)$}|-{$(current bounding box.south west)!0.98!(current bounding box.north west)$}) node[
  scale=0.6,
  anchor=north,
  text=black,
  rotate=0.0
]{Shift};
\end{tikzpicture}
